# Supplementary material for: Restore Anything Model via Efficient Degradation Adaptation
Source: arXiv:2407.13372 source file (2024-12-18)
Supplement: Supplementary file 2 [file supp_capacity.tex]

\begin{table}[t]
    \centering
    \footnotesize
    \setlength\tabcolsep{1.8pt}
    \setlength{\extrarowheight}{0.5pt}
    \caption{\textit{Network Capacity and Complexity Analysis on Deraining.} Comparison of PSNR, model parameters, and FLOPs, highlighting the balance between network capacity and computational efficiency. FLOPs are computed for $224\times224$ input images using an NVIDIA Tesla A100 (40G) GPU.}
    \vspace{-3mm}
    \label{tab:supp_capacity}
    \begin{tabularx}{\columnwidth}{X*{5}{c}}
    % \begin{tabularx}{\textwidth}{X*{3}{c}}
        \toprule
        Method  &Blocks &PSNR (dB, $\uparrow$) &Params. ($\downarrow$) & FLOPs ($\downarrow$) \\
        \midrule
        PromptIR~\cite{potlapalli2023promptir}(Base) & [4,6,6,8] &37.04 & 35.6M & 132G \\
        Base (No Prompt)& [4,6,6,8] & 36.74 & 32.2M & 117G \\
        Base (Fix-Prompt) & [4,6,6,8] & 36.85 & - & -  \\
        \midrule
        Base (No Prompt) & [3,5,5,7] & 36.84 & 29.1M & 101G \\
        Base (No Prompt) & [2,4,4,6] & 36.76 & 26.0M & 85G \\
        Base (No Prompt) & [1,3,3,5] & 36.63 & 22.9M & 68G \\
        \midrule
        \ourmethod(\textit{ours}) & [3,5,5,7] &\textcolor{tabred}{\textbf{37.79}} & \textcolor{tabred}{\textbf{6.3M}} & \textcolor{tabred}{\textbf{19G}} \\ 
        \bottomrule
    \end{tabularx}
    \vspace{-2.4em}
\end{table}
