# Supplementary material for: Restore Anything Model via Efficient Degradation Adaptation
Source: arXiv:2407.13372 source file (2024-12-18)
Supplement: Supplementary file 3 [file supp_inference.tex]

\begin{table}[t]
    \centering
    \footnotesize
    \setlength\tabcolsep{2.5pt}
    \caption{Full \textbf{inference time} comparison under the 3-degradation all-in-one IR setting. The lower the better.}
    \vspace{-2mm}
    \label{tab:inferencetime}
    \setlength{\extrarowheight}{2pt}
    \setlength\tabcolsep{4pt}
    \scalebox{1}{
    \begin{tabularx}{\columnwidth}{X*{4}{c}}
    % \begin{tabularx}{\textwidth}{X*{3}{c}}
        \toprule
        Task  & Num. Samples & PromptIR~\cite{potlapalli2023promptir} & \ourmethod (Ours)  \\
        \midrule
        Denoising ($\sigma=15$)& 68 & 41s & 30s \\ 
        Denoising ($\sigma=25$)& 68 & 41s & 30s \\ 
        Denoising ($\sigma=50$)& 68 & 42s & 30s \\ 
        \midrule
        Deraining & 100 & 60s & 43s \\ 
        \midrule
        Dehazing & 500 & 416s & 274s\\
        \midrule
        Frames Per Second & - & 1.34 & 1.97\\
        \bottomrule        
    \end{tabularx}
    }
    \vspace{0mm}
\end{table}
