# Supplementary material for: Restore Anything Model via Efficient Degradation Adaptation
Source: arXiv:2407.13372 source file (2024-12-18)
Supplement: Supplementary file 4 [file supp_mixdeg.tex]

\begin{table}[t]
    \centering
    \footnotesize
    \setlength\tabcolsep{1pt} 
    \caption{\textbf{Mixed degradation} result with the CDD-11~\cite{guo2024onerestore} dataset.}
    \vspace{-2mm}
    \label{tab:supp_mix}
    \begin{tabularx}{\columnwidth}{>{\raggedright\arraybackslash}m{3.1cm}c@{\hskip 10pt}c@{\hskip 20pt}c@{\hskip 8pt}c}
        \toprule
        \multirow{2}{*}{\textbf{Method}} & \multicolumn{2}{c}{low-light+haze+rain} & \multicolumn{2}{c}{low-light+haze+snow} \\
        \cmidrule(r){2-3} \cmidrule(r){4-5} % 短线范围优化
        & PSNR & SSIM & PSNR & SSIM \\
        \midrule
        AirNet~\cite{li2022airnet} & 21.80 & .708 & 22.23 & .725 \\
        TransWeather~\cite{valanarasu2022transweather} & 21.55 & .678 & 21.01 & .655 \\
        % WeatherDiff & 21.23 & .716 & 21.03 & .698 \\
        PromptIR~\cite{potlapalli2023promptir} & 23.51 & .752 & 23.33 & .747 \\
        \ourmethod (Ours) & \textcolor{tabred}{\textbf{24.54}} & \textcolor{tabred}{\textbf{.783}} & \textcolor{tabred}{\textbf{24.67}} & \textcolor{tabred}{\textbf{.790}} \\
        % OneRestore & 25.18 & .795 & 25.28 & .797 \\
        \bottomrule
    \end{tabularx}
    \vspace{-3mm}
\end{table}
