# Supplementary material for: Restore Anything Model via Efficient Degradation Adaptation
Source: arXiv:2407.13372 source file (2024-12-18)
Supplement: Supplementary file 5 [file supp_unseen.tex]

\begin{table}[t]
    \centering
    \footnotesize
    \setlength\tabcolsep{2.0pt}
    \caption{Unseen \textbf{Desnowing} comparison with the CSD~\cite{chen2021all} dataset.}
    \vspace{-2mm}
    \label{tab:supp_unseen}
    \setlength{\extrarowheight}{2pt}
    \setlength\tabcolsep{4pt}
    \scalebox{1}{
    \begin{tabularx}{\columnwidth}{X*{4}{c}}
    % \begin{tabularx}{\textwidth}{X*{3}{c}}
        \toprule
        Method  & AirNet~\cite{li2022airnet} & PromptIR~\cite{potlapalli2023promptir} & \ourmethod (Ours)  \\
        \midrule
        PSNR & 19.32 & 20.47 & \textcolor{tabred}{\textbf{21.54}} \\ 
        SSIM & .733 & .764 & \textcolor{tabred}{\textbf{.781}} \\ 
        \bottomrule        
    \end{tabularx}
    }
    \vspace{-1mm}
\end{table}
